# Supplementary material for: Efficient parallel solver for rarefied gas flow using GSIS
Source: arXiv:2310.18916 source file (2024-04-16)
Supplement: Supplementary file 1 [file appendix_numerical_method.tex]

\section{Implicit treatment of source terms in macroscopic equations}\label{appendix:source_term}

Taking the 2D two-temperature macroscopic equation \eqref{eq:macroscopic_equation_2} as an example, the conservative variables can be obtained as:
\begin{equation}
\bm{W}=
\begin{bmatrix}
\rho \\
\rho u_x \\
\rho u_y \\
E\\
E_r\\
\end{bmatrix},\;
\bm{F}_c=
\begin{bmatrix}
\rho u_n\\
\rho u_xu_n+n_xp_t\\
\rho u_yu_n+n_yp_t\\
u_n (E+p_t)\\
u_nE_r\\
\end{bmatrix}, \;
\bm{F}_v=
\begin{bmatrix}
0\\
n_x\sigma_{xx}+n_y\sigma_{xy}\\
n_x\sigma_{yx}+n_y\sigma_{yy}\\
n_x\Theta_{x}+n_y\Theta_{y}\\
n_xq_{x,r}+n_yq_{y,r}\\
\end{bmatrix},\;
\bm{Q}=
\begin{bmatrix}
0\\
0\\
0\\
0\\
{\frac{E_{tr}-E_{r}}{Z_r\tau}}
\end{bmatrix},
\end{equation}
with 
$\Theta_{x} =u_x\sigma_{xx}+u_y\sigma_{xy}+q_x$ and
$\Theta_{y} =u_x\sigma_{yx}+u_y\sigma_{yy}+q_y$. 
Here, $u_n = u_x n_x + u_y n_y$ is defined as the scalar product of the macro velocity vector and the unit normal vector of the face. The total energy in the macroscopic system is obtained by adding its internal energy to its kinetic energy. Thus we can define those components as follows,
 \begin{equation}
E_{t}=\frac{3}{2}\rho T_{t}+\frac{1}{2}\rho u^2,\;
(E_{r},E_{tr})=\frac{d_r}{2}\rho (T_{r},T),\; E=E_t + E_r=\rho\left(c_vT+\frac{1}{2}u^2\right).
\end{equation}
we provide an approximation procedure for the source term Jacobi matrix in the Cartesian coordinate system. It should be noted that the rotational collision numbers $Z_r$ used here are all constants. If the rotational collision number is temperature-dependent, a new derivation would be required. The Jacobi matrix $T$ represents the derivative of the source term $Q$. The matrix can be further approximated by only keeping its main diagonal elements, which leads to diagonalization of the matrix as follows:
\begin{equation}
\mathbf{T} = \frac{\partial \mathbf{Q}}{\partial \mathbf{W}} = 
\left[
\begin{matrix}
0 & 0 & 0 & 0 & 0 \\
0 & 0 & 0 & 0 & 0 \\
0 & 0 & 0 & 0 & 0 \\
0 & 0 & 0 & 0 & 0 \\
\frac{\partial Q(5)}{\partial W(1)} & \frac{\partial Q(5)}{\partial W(2)} & \frac{\partial Q(5)}{\partial W(3)} & \frac{\partial Q(5)}{\partial W(4)} & \frac{\partial Q(5)}{\partial W(5)} \\
\end{matrix}
\right]\approx
\left[
\begin{matrix}
0 & 0 & 0 & 0 & 0 \\
0 & 0 & 0 & 0 & 0 \\
0 & 0 & 0 & 0 & 0 \\
0 & 0 & 0 & 0 & 0 \\
0 & 0 & 0 & 0 & \frac{\partial Q(5)}{\partial W(5)} \\
\end{matrix}
\right],
\end{equation}
where
\begin{equation}
\begin{aligned}
\frac{\partial Q(5)}{\partial E_r}&=\frac{\partial \left(\frac{d_r}{2}\frac{\rho(T-T_r)}{Z_r\tau}\right)}{\partial \left(\frac{d_r}{2}\rho T_r\right)}=\frac{1}{Z_r}\frac{\partial \left(\frac{\rho(T-T_r)}{\tau}\right)}{\partial \left(\rho T_r\right)}\\
&=\frac{1}{Z_r}\left[\frac{\partial \left(\rho T-\rho T_r\right)}{\partial \rho T_r}\cdot\frac{1}{\tau}-\frac{\rho(T-T_r)}{\tau^2}\cdot\frac{\partial \tau}{\partial T_t}\cdot\frac{\partial T_t}{\partial \rho T_r}\right]\\
&=-\frac{3}{(3+dr)Z_r\tau}+\frac{2(T-T_r)}{3\tau^2}\cdot\frac{\partial \tau}{\partial T_t},
\end{aligned}
\end{equation}
where those derivative terms can be expressed as:
\begin{equation}
\frac{\partial T_t}{\partial E_r}=-\frac{2}{3\rho},\quad \frac{\partial (\rho T)}{\partial ( \rho T_r)} = \frac{d_r}{3+d_r}, \quad \frac{\partial \tau}{\partial T_t}=(\omega-1)\frac{T_t^{\omega-2}}{\rho}.
\end{equation}

The approximate Jacobi matrix indicates that the non-principal diagonal elements are all zero, and the solution of the rotational energy relaxation equation is approximated by decoupling.
